# Supplementary material for: Learning Energy Based Inpainting for Optical Flow
Source: arXiv:1811.03721 source file (2018-11-09)
Supplement: Supplementary file 3 [file supplementary.tex]

Our supplementary material provides the full backward algorithm for inpainting 
optical flow with Total Generalized Variation~\cite{Bredies2010} of 
second order, according to \Eq (2) of the main paper. 
We first repeat the objective in its discretized form:
\begin{equation}\label{eq:tgv_disc_supp}
\min_{u_i}\min_{w_{i}=(w_{i,0},w_{i,1}\!)\trans}
\|\sqrt{W} (D u_i - w_{i})\|_\delta +
\beta ( \|D w_{i,0}\|_\delta + \|D w_{i,1} \|_\delta ) +
\|u_i-\hat{u}_i\|_c. 
\end{equation}
Here, the auxiliary variables $w_{i,j}\!\in\!\R^{NM}$, $i,j \in\{0,1\}$ 
denote the diffusion tensor and the norm $\|\cdot\|_c$ denotes 
the $\ell_1$ norm weighted by the confidence $c$. 
\section{Optimization Layer for TGV}
For completeness we repeat the forward algorithm first. 
\begin{align}
  (u_i^{k+0.5},w_{i}^{k+1})\trans &:= (v_i^k,q_{i}^k)\trans - B\trans \frac{V_\beta}{\max( 1, |\sqrt{V}B (v_i^k,q_{i}^k)\trans|_2/\delta ) } B (v_i^k,q_{i}^k)\trans \label{eq:fg_u05}
  \\
  u_i^{k+1} &:= \left\{
  \begin{array}{cl}
  u_i^{k+0.5} - c\; &\textrm{if } u_i^{k+0.5} - c > \hat{u}_i \\
  u_i^{k+0.5} + c\; &\textrm{if } u_i^{k+0.5} + c < \hat{u}_i \\
  \hat{u}_i\; & \textrm{else}
  \end{array}\right.\label{eq:fg_u1}
  \\
  (v_{i}^{k+1},q_{i}^{k+1})\trans &:= (u_{i}^{k+1},w_{i}^{k+1})\trans + \frac{t^k-1}{t^{k+1}} (u_{i}^{k+1},w_{i}^{k+1})\trans - (u_{i}^{k},w_{i}^{k})\trans), \label{eq:fg_v1}
\end{align}
%  \end{linenomath}
%
Now, analogue to the TV case we can define a single iteration of the 
backward path for TGV inpainting as follows: 
\begin{align}
  \frac{\partial f}{\partial \hat{u}_i} &:= \frac{\partial f}{\partial \hat{u}_i} + \frac{\partial f}{\partial u_i^{k+1}} \textrm{ if } c < |\hat{u}_i-u_i^{k+0.5} | \label{eq:dguhat}
  \\
  \frac{\partial f}{\partial c} &:= \frac{\partial f}{\partial c} + \textrm{sign}(\hat{u}_i-u_i^{k+0.5}) \frac{\partial f}{\partial u_i^{k+1}} \textrm{ if } c \geq |\hat{u}_i-u_i^{k+0.5}| \label{eq:dgc}
%  \\
\end{align}
\begin{align}
  \frac{\partial f}{\partial u_i^{k+0.5}} &:=
  \left\{
  \begin{array}{cl}
  \frac{\partial f}{\partial u_i^{k+1}}\; & \textrm{if } c \geq |\hat{u}_i-u_i^{k+0.5}|
  %&\textrm{if } x^{k+0.5} - c > b \textrm{ or } x^{k+0.5} + c < b
  \\
  0 & \textrm{else}
  \end{array}\right. \label{eq:dgu05}
  \\
  %\left(\frac{\partial}{\partial v_i^{k}}, \frac{\partial f}{\partial q_i^{k}}\right)\trans
  %\left(\frac{\partial f}{\partial v_i^{k}} \right. & \left. \frac{\partial f}{\partial q_i^{k}} \right)\trans 
  \vecII{\frac{\partial f}{\partial v_i^{k}}}{\frac{\partial f}{\partial q_i^{k}}} &
  := \!\left(\! I\!-\! \vecII{\frac{\partial}{\partial v_i^{k}}}{\frac{\partial}{\partial q_i^{k}}} \!\!\left(\!\! \frac{V_\beta}{\scriptstyle \max\left( 1, \left|\sqrt{V}B \vecII{v_i^k}{q_i^k}\right|_2/\delta \right) } B \vecII{v_i^k}{q_i^k} \!\!\right)\trans \right) \!B \vecII{\frac{\partial f}{\partial u_i^{k+0.5}}}{\frac{\partial f}{\partial w_i^{k+1}}} \label{eq:update_dgv}
  \raisetag{1.15cm}
  \\
  \frac{\partial f}{\partial V_\beta} & := \frac{\partial f}{\partial V_\beta} + \frac{\partial}{\partial V_\beta} 
  \!\left(\! \frac{V_\beta}{\scriptstyle \max\left( 1, \left|\sqrt{V}B \vecII{v_i^k}{q_i^k}\right|_2/\delta \right) } B \vecII{v_i^k}{q_i^k} \!\!\right)\trans \!B \vecII{\frac{\partial f}{\partial u_i^{k+0.5}}}{\frac{\partial f}{\partial w_i^{k+1}}}\label{eq:update_dgw}
  %\left(\frac{V}{\max( 1, |\sqrt{V}D v_i^k|_2/\delta ) } D v_i^k\right)\trans D \frac{\partial f}{\partial u_i^{k+0.5}}\label{eq:update_dw}
%\end{align}
\\
%\begin{align}
  \left(\frac{\partial f}{\partial u_i^{k}}, \right. & \left. \frac{\partial f}{\partial w_i^{k}}\right)\trans := \left(\frac{\partial f}{\partial u_i^{k}},\frac{\partial f}{\partial w_i^{k}}\right)\trans + \left(1+\frac{t^{k-1}-1}{t^{k}}\right) \left(\frac{\partial f}{\partial v_i^{k}}, \frac{\partial f}{\partial q_i^{k}}\right)\label{eq:dgu_k}
  \\
  \left(\frac{\partial f}{\partial u_i^{k\!-\!1}}, \right. \!\! & \left.\frac{\partial f}{\partial w_i^{k\!-\!1}}\right)\trans \!:=\! -\frac{t^{k-1}-1}{t^{k}} \left(\frac{\partial f}{\partial v_i^{k}}, \frac{\partial f}{\partial q_i^{k}}\right)\trans. \label{eq:dgu_minus1}
  %\frac{\partial f}{\partial u_i^{k-1}}\textrm{ (used in the line above at iteration k-1) }.\label{eq:du_minus1}
  \end{align}
%  \end{linenomath}
%
As before for the TV case, we use the outer products in 
(\ref{eq:update_dgv}, \ref{eq:update_dgw}) for a compact notation. 
%In our implementation,
Again, our implementation exploits the extreme sparsity of 
the resulting matrices. 
To achieve memory and numerical efficiency, the algorithm operates similar 
to the TV case and we refer to the main paper for a description of the procedure. 
%Algorithmically we operate in the same manner as described for the TV case. 
%
%In both cases we set $\delta$ to $0.1$. 
%
The only exception is that the gradient \wrt $\beta$ is computed for each 
pixel and finally has to be summed over all the pixels. 
%Please note that instead of learning a single scalar $\beta$ the algorithm
%can be directly extended to  
%a diffusion tensor , to be applied on the auxilliary variables $w_0,w_1$. 
%
Finally, please recall that the algorithm can be easily extended to learn 
a pixel-wise diffusion tensor for the auxilliary variables $w_0,w_1$
instead of a single scalar $\beta$. 
